# Supplementary material for: Counting zeros of Dedekind zeta functions
Source: arXiv:2102.04663 ancillary file (2021-05-03)
Supplement: Supplementary file 1 [file Maple_code.pdf]

$$\begin{aligned} &> \text{sigma} := (c, r, y) \rightarrow c + r \cdot \cos(y) \\ &\quad \sigma := (c, r, y) \mapsto c + r \cdot \cos(y) \end{aligned} \quad (1)$$

$$\begin{aligned} &> \text{sigma1} := (c, r) \rightarrow c + (c - 1/2)^2 / r \\ &\quad \sigma^I := (c, r) \mapsto c + \frac{\left(c - \frac{1}{2}\right)^2}{r} \end{aligned} \quad (2)$$

$$\begin{aligned} &> \text{delta} := (c, r) \rightarrow 2 \cdot c - \text{sigma1}(c, r) - 1/2 \\ &\quad \delta := (c, r) \mapsto 2 \cdot c - \sigma^I(c, r) - \frac{1}{2} \end{aligned} \quad (3)$$

$$\begin{aligned} &> \text{Lstar} := (c, r, y, j) \\ &\quad \rightarrow 2 \cdot r \cdot \sin(y) - 4 + 7/19 \cdot ((j + c + r \cdot \cos(y))^2 + (r \cdot \sin(y) - 2)^2) \\ &\quad Lstar := (c, r, y, j) \mapsto 2 \cdot r \cdot \sin(y) - 4 + \frac{7 \cdot (j + c + r \cdot \cos(y))^2}{19} + \frac{7 \cdot (r \cdot \sin(y) - 2)^2}{19} \end{aligned} \quad (4)$$

$$\begin{aligned} &> \text{theta} := (c, r, t) \\ &\quad \rightarrow \text{piecewise}(t \geq c + r, 0, \\ &\quad \quad c - r \leq t \text{ and } t \leq c + r, \arccos((t - c) / r), \\ &\quad \leq c - r, \text{Pi}); \\ &\quad \theta := (c, r, t) \mapsto \begin{cases} 0 & c + r \leq t \\ \arccos\left(\frac{t - c}{r}\right) & c - r \leq t \leq c + r \\ \pi & t \leq c - r \end{cases} \end{aligned} \quad (5)$$

$$\begin{aligned} &> \text{kappa1} := (\eta, c, r) \\ &\quad \rightarrow \text{int}((1 + \eta - \text{sigma}(c, r, y)) / 2, y = \text{theta}(c, r, 1 + \eta) \dots \text{theta}(c, r, -\eta)) \\ &\quad + \text{int}((1 - 2 \cdot \text{sigma}(c, r, y)) / 2, y = \text{theta}(c, r, -\eta) \dots \text{Pi}) \\ &\quad \kappa^I := (\eta, c, r) \mapsto \int_{\theta(c, r, \eta + 1)}^{\theta(c, r, -\eta)} \left( \frac{1}{2} + \frac{\eta}{2} - \frac{\sigma(c, r, y)}{2} \right) dy + \int_{\theta(c, r, -\eta)}^{\pi} \left( \frac{1}{2} - \sigma(c, r, y) \right) dy \end{aligned} \quad (6)$$

$$\begin{aligned} &> \text{kappa2} := (J1, c, r) \\ &\quad \rightarrow \text{Pi} / (4 \cdot J1) \cdot (\ln(\text{Zeta}(c + r)) \\ &\quad \quad + 2 \cdot \text{sum}(\ln(\text{Zeta}(c + r \cdot \cos((\text{Pi} \cdot j) / (2 \cdot J1))))), j = 1 \dots J1 - 1) \end{aligned}$$

$$\kappa^2 := (J1, c, r) \mapsto \frac{\pi \cdot \left( \ln(\zeta(c+r)) + 2 \cdot \left( \sum_{j=1}^{J1-1} \ln \left( \zeta \left( c + r \cdot \cos \left( \frac{\pi \cdot j}{2 \cdot J1} \right) \right) \right) \right) \right)}{4 \cdot J1} \quad (7)$$

> kappa3:=(J2,c,r)  
 ->(Pi-theta(c,r,1-c))/(2\*J2)\*(ln(Zeta(1-c+r))  
 + 2\*sum(ln(Zeta(1-c-r\*cos((Pi\*j)/(J2)+(1-j/J2)\*  
 theta(c,r,1-c)))) ,j=1..(J2-1)))

$$\kappa^3 := (J2, c, r) \mapsto \frac{1}{2 \cdot J2} \left( (\pi - \theta(c, r, 1-c)) \cdot \left( \ln(\zeta(1-c+r)) + 2 \cdot \left( \sum_{j=1}^{J2-1} \ln \left( \zeta \left( 1-c - r \cdot \cos \left( \frac{\pi \cdot j}{J2} + \left( 1 - \frac{j}{J2} \right) \cdot \theta(c, r, 1-c) \right) \right) \right) \right) \right) \right) \quad (8)$$

> kappa4:=(eta,c,r)  
 ->1/4\*int((1+eta-sigma(c,r,y))\*Lstar(c,r,y,1),  
 y=theta(c,r,1+eta)..theta(c,r,-eta))

$$\kappa^4 := (\eta, c, r) \mapsto \frac{\left( \int_{\theta(c, r, \eta+1)}^{\theta(c, r, -\eta)} (1 + \eta - \sigma(c, r, y)) \cdot Lstar(c, r, y, 1) dy \right)}{4} \quad (9)$$

> kappa5:=(eta,c,r)  
 ->1/4\*int((1-2\*sigma(c,r,y))\*Lstar(c,r,y,1),  
 y=theta(c,r,-eta)..theta(c,r,-1/2))

$$\kappa^5 := (\eta, c, r) \mapsto \frac{\left( \int_{\theta(c, r, -\eta)}^{\theta \left( c, r, -\frac{1}{2} \right)} (1 - 2 \cdot \sigma(c, r, y)) \cdot Lstar(c, r, y, 1) dy \right)}{4} \quad (10)$$

> C1 := (c,r,eta) -> kappa1(eta,c,r)/(Pi\*ln(r/(c - 1/2)))

$$C1 := (c, r, \eta) \mapsto \frac{\kappa^1(\eta, c, r)}{\pi \cdot \ln \left( \frac{r}{c - \frac{1}{2}} \right)} \quad (11)$$

> evalf(C1(1.000011314, 1.064340602, 4.2826451\*10^(-6)))

$$0.2273699052 \quad (12)$$

> evalf(C1(1.042877508, 1.259860485, 0.01737451737))

$$(13)$$

0.2449270413

(13)

> evalf(C1(1.079779637, 1.410370323,  
0.03441682600))

0.2630376946

(14)

> evalf(C1(1.114294066, 1.538391756,  
0.05247813411))

0.2803185714

(15)

> evalf(C1(1.145720440, 1.645584376,  
0.07107039918))

0.2958905284

(16)

> C2 := (c, r, eta, T, J1, J2)

→  $\frac{1}{25 * T} + \frac{2}{\text{Pi}} * \ln(\text{Zeta}(\text{sigma1}(c, r)))$

+  $\frac{640 * \text{delta}(c, r) - 112}{1536 * (3 * T - 1)}$

+ max( $0, \frac{856 * \text{delta}(c, r) - 151}{1536 * (3 * T + 2)}$

-  $\frac{640 * \text{delta}(c, r) - 112}{1536 * (3 * T - 1)}$ ) +  $\frac{1}{2^{10}}$

+  $1 / (\text{Pi} * \ln(r / (c - 1/2))) * \left( 0.5 * (\ln(\text{Zeta}(1 + \text{eta}))) \right.$

+  $\ln(\text{Zeta}(c))) * \left( \text{theta}(c, r, 1 + \text{eta}) - \frac{\text{Pi}}{2} \right)$

+  $\frac{\text{Pi} * \ln(\text{Zeta}(c))}{4 * J1} + \text{kappa2}(J1, c, r) \Big)$

+  $1 / (\text{Pi} * \ln(r / (c - 1/2))) * \left( 0.5 * (\ln(\text{Zeta}(1 + \text{eta}))) \right.$

+  $\ln(\text{Zeta}(c))) * (\text{theta}(c, r, 1 - c) - \text{theta}(c, r,$

-eta)) +  $\frac{(\text{Pi} - \text{theta}(c, r, 1 - c)) * \ln(\text{Zeta}(c))}{2 * J2}$

+  $\text{kappa3}(J2, c, r) \Big)$

+  $1 / (\text{Pi} * \ln(r / (c - 1/2))) * \left( \ln(\text{Zeta}(1 + \text{eta})) \right.$

$$\begin{aligned}
& * (\text{theta}(c, r, -\text{eta}) - \text{theta}(c, r, 1 + \text{eta})) \\
& + \max\left(0, \frac{\text{kappa4}(\text{eta}, c, r) + \text{kappa5}(\text{eta}, c, r)}{T + 2}\right) + \text{Pi} \\
& * \ln(\text{Zeta}(c) / \text{Zeta}(2 * c)) \Big)
\end{aligned}$$

$$C2 := (c, r, \eta, T, J1, J2) \mapsto \frac{1}{25 \cdot T} + \frac{2 \cdot \ln(\zeta(\sigma I(c, r)))}{\pi} + \frac{640 \cdot \delta(c, r) - 112}{4608 \cdot T - 1536} + \max\left(0, \quad (17)$$

$$\frac{856 \cdot \delta(c, r) - 151}{4608 \cdot T + 3072} - \frac{640 \cdot \delta(c, r) - 112}{4608 \cdot T - 1536} \Big) + \frac{1}{1024}$$

$$+ \frac{1}{\pi \cdot \ln\left(\frac{r}{c - \frac{1}{2}}\right)} \left(0.5 \cdot (\ln(\zeta(\eta + 1)) + \ln(\zeta(c))) \cdot \left(\theta(c, r, \eta + 1) - \frac{\pi}{2}\right)\right)$$

$$+ \frac{\pi \cdot \ln(\zeta(c))}{4 \cdot J1} + \kappa2(J1, c, r) \Big) + \frac{1}{\pi \cdot \ln\left(\frac{r}{c - \frac{1}{2}}\right)} \left(0.5 \cdot (\ln(\zeta(\eta + 1))\right.$$

$$+ \ln(\zeta(c))) \cdot (\theta(c, r, 1 - c) - \theta(c, r, -\eta)) + \frac{(\pi - \theta(c, r, 1 - c)) \cdot \ln(\zeta(c))}{2 \cdot J2}$$

$$+ \kappa3(J2, c, r) \Big) + \frac{1}{\pi \cdot \ln\left(\frac{r}{c - \frac{1}{2}}\right)} \left(\ln(\zeta(\eta + 1)) \cdot (\theta(c, r, -\eta) - \theta(c, r, \eta + 1))\right)$$

$$+ \max\left(0, \frac{\kappa4(\eta, c, r) + \kappa5(\eta, c, r)}{T + 2}\right) + \pi \cdot \ln\left(\frac{\zeta(c)}{\zeta(2 \cdot c)}\right) \Big)$$

$$\begin{aligned}
> \text{evalf}(C2(1.000011314, 1.064340602, 4.2826451 \cdot 10^{\wedge} \\
(-6), 1, 64, 39)) \\
23.02526263 \quad (18)
\end{aligned}$$

$$\begin{aligned}
> \text{evalf}(C2(1.042877508, 1.259860485, 0.01737451737, \\
1, 64, 39)) \\
6.665567830 \quad (19)
\end{aligned}$$

$$\begin{aligned}
> \text{evalf}(C2(1.079779637, 1.410370323, \\
0.03441682600, 1, 64, 39)) \\
5.220309511 \quad (20)
\end{aligned}$$

$$\begin{aligned}
> \text{evalf}(C2(1.114294066, 1.538391756, \\
0.05247813411, 1, 64, 39)) \\
4.435200196 \quad (21)
\end{aligned}$$

$$\begin{aligned}
> \text{evalf}(C2(1.145720440, 1.645584376,
\end{aligned}$$

$$0.07107039918, 1, 64, 39))$$

$$3.938877656 \quad (22)$$

$$> \text{evalf}(C2(1.000011314, 1.064340602, 4.2826451 \cdot 10^{\wedge}(-6), 1, 64, 39) - 0.00001 \cdot \ln(3/(2 \cdot \text{Pi})))$$

$$23.02527002 \quad (23)$$

$$> \text{evalf}(C2(1.042877508, 1.259860485, 0.01737451737, 1, 64, 39) - 0.00001 \cdot \ln(3/(2 \cdot \text{Pi})))$$

$$6.665575223 \quad (24)$$

$$> \text{evalf}(C2(1.079779637, 1.410370323, 0.03441682600, 1, 64, 39) - 0.00001 \cdot \ln(3/(2 \cdot \text{Pi})))$$

$$5.220316904 \quad (25)$$

$$> \text{evalf}(C2(1.114294066, 1.538391756, 0.05247813411, 1, 64, 39) - 0.00001 \cdot \ln(3/(2 \cdot \text{Pi})))$$

$$4.435207589 \quad (26)$$

$$> \text{evalf}(C2(1.145720440, 1.645584376, 0.07107039918, 1, 64, 39) - 0.00001 \cdot \ln(3/(2 \cdot \text{Pi})))$$

$$3.938885049 \quad (27)$$

*> # the term "-0.00001 ln(3/2pi) > 0" is added because the C1 term may be negative when T is "small".*  
*For instance, when  $T + 2 > 2 \pi$ ,  $0.2273699053 n_K \ln((T + 2)/2 \pi) < 0.22737 n_K \ln((T + 2)/2 \pi)$ .*  
*However, when  $3 \leq T + 2 \leq 2 \pi$ , we have*  

$$0.2273699053 n_K \ln((T + 2)/2 \pi)$$

$$\leq 0.22736 n_K \ln((T + 2)/2 \pi)$$

$$= 0.22737 n_K \ln((T + 2)/2 \pi) - 0.00001 n_K \ln((T + 2)/2 \pi)$$

$$\leq 0.22737 n_K \ln((T + 2)/2 \pi) - 0.00001 n_K \ln(3/2 \pi).$$

$$> \text{evalf}(C2(1.000011314, 1.064340602, 4.2826451 \cdot 10^{\wedge}(-6), 10, 64, 39))$$

$$22.97203394 \quad (28)$$

$$> \text{evalf}(C2(1.042877508, 1.259860485, 0.01737451737, 10, 64, 39))$$

$$6.603969949 \quad (29)$$

$$> \text{evalf}(C2(1.079779637, 1.410370323, 0.03441682600, 10, 64, 39))$$

$$5.152508342 \quad (30)$$

$$> \text{evalf}(C2(1.114294066, 1.538391756, 0.05247813411, 10, 64, 39))$$

$$4.362137551 \quad (31)$$

$$\begin{aligned} &> \text{evalf}(C2(1.145720440, 1.645584376, \\ &\quad 0.07107039918, 10, 64, 39)) \\ &\quad 3.861358666 \end{aligned} \quad (32)$$

$$\begin{aligned} &> D2 := (c, r, \eta, T, J1, J2) \\ &\quad \rightarrow C2(c, r, \eta, T, J1, J2) + (C1(c, r, \eta) \\ &\quad \cdot \left( \ln \left( \frac{1 + \left( \frac{2}{T} \right)}{(2 \cdot \text{Pi})} \right) \right) + 0.25 \\ &\quad - 0.00001 \cdot \ln(3 / (2 \cdot \text{Pi})) \\ &\quad D2 := (c, r, \eta, T, J1, J2) \mapsto C2(c, r, \eta, T, J1, J2) + C1(c, r, \eta) \cdot \ln \left( \frac{1 + \frac{2}{T}}{2 \cdot \pi} \right) + 0.25 \\ &\quad - 0.00001 \ln \left( \frac{3}{2 \pi} \right) \end{aligned} \quad (33)$$

> # the term "-0.00001 ln(3/2pi)>0" is added for the exact same reason above.

$$\begin{aligned} &> \text{evalf}(D2(1.000011314, 1.064340602, 4.2826451 \cdot 10^{\wedge} \\ &\quad (-6), 1, 64, 39)) \\ &\quad 23.10717607 \end{aligned} \quad (34)$$

$$\begin{aligned} &> \text{evalf}(D2(1.042877508, 1.259860485, 0.01737451737, \\ &\quad 1, 64, 39)) \\ &\quad 6.734501895 \end{aligned} \quad (35)$$

$$\begin{aligned} &> \text{evalf}(D2(1.079779637, 1.410370323, \\ &\quad 0.03441682600, 1, 64, 39)) \\ &\quad 5.275855008 \end{aligned} \quad (36)$$

$$\begin{aligned} &> \text{evalf}(D2(1.114294066, 1.538391756, \\ &\quad 0.05247813411, 1, 64, 39)) \\ &\quad 4.477970550 \end{aligned} \quad (37)$$

$$\begin{aligned} &> \text{evalf}(D2(1.145720440, 1.645584376, \\ &\quad 0.07107039918, 1, 64, 39)) \\ &\quad 3.970136210 \end{aligned} \quad (38)$$

$$\begin{aligned} &> \text{evalf}(D2(1.000011314, 1.064340602, 4.2826451 \cdot 10^{\wedge} \\ &\quad (-6), 10, 64, 39)) \\ &\quad 22.84561044 \end{aligned} \quad (39)$$

$$\begin{aligned} &> \text{evalf}(D2(1.042877508, 1.259860485, 0.01737451737, \\ &\quad 10, 64, 39)) \\ &\quad 6.448479636 \end{aligned} \quad (40)$$

$$\begin{aligned} &> \text{evalf}(D2(1.079779637, 1.410370323, \\ &\quad 0.03441682600, 10, 64, 39)) \\ &\quad \quad \quad 4.967034837 \end{aligned} \quad (41)$$

$$\begin{aligned} &> \text{evalf}(D2(1.114294066, 1.538391756, \\ &\quad 0.05247813411, 10, 64, 39)) \\ &\quad \quad \quad 4.148054596 \end{aligned} \quad (42)$$

$$\begin{aligned} &> \text{evalf}(D2(1.145720440, 1.645584376, \\ &\quad 0.07107039918, 10, 64, 39)) \\ &\quad \quad \quad 3.621495471 \end{aligned} \quad (43)$$

$$\begin{aligned} &> C3 := (c, r, \eta, T) \\ &\quad \rightarrow 2.5 \\ &\quad + 1 / (\text{Pi} * \ln(r / (c - 1/2))) * \left( \text{Pi} * \ln\left(1 + \frac{2}{T}\right) \right. \\ &\quad \quad \left. + (\text{theta}(c, r, -\eta) - \text{theta}(c, r, 1 + \eta)) * \ln(3) \right) \\ &\quad + \max\left(0, 1 / (\text{Pi} * \ln(r / (c - 1/2))) * \left( \frac{1}{2 * (T + 2)} \right. \right. \\ &\quad \quad * (\text{int}(\text{Lstar}(c, r, y, -1), y = 0 .. \text{theta}(c, r, 1 + \eta)) \\ &\quad \quad + \text{int}(\text{Lstar}(c, r, y, 1), y = \text{theta}(c, r, 1 + \eta) .. \text{theta}(c, r, -\eta)) \\ &\quad \quad + \text{int}(\text{Lstar}(c, r, y, -1), y = \text{theta}(c, r, -\eta) .. \text{Pi})) \left. \right) \\ &C3 := (c, r, \eta, T) \mapsto 2.5 + \frac{\pi \cdot \ln\left(1 + \frac{2}{T}\right) + (\theta(c, r, -\eta) - \theta(c, r, \eta + 1)) \cdot \ln(3)}{\pi \cdot \ln\left(\frac{r}{c - \frac{1}{2}}\right)} \end{aligned} \quad (44)$$

$$\begin{aligned} &+ \max\left(0, \frac{1}{\pi \cdot \ln\left(\frac{r}{c - \frac{1}{2}}\right) \cdot (2 \cdot T + 4)} \left( \int_0^{\theta(c, r, \eta + 1)} \text{Lstar}(c, r, y, -1) dy + \right. \right. \\ &\quad \left. \left. \int_{\theta(c, r, \eta + 1)}^{\theta(c, r, -\eta)} \text{Lstar}(c, r, y, 1) dy + \int_{\theta(c, r, -\eta)}^{\pi} \text{Lstar}(c, r, y, -1) dy \right) \right) \end{aligned}$$

$$\begin{aligned} &> \text{evalf}(C3(1.000011314, 1.064340602, 4.2826451 * 10^ \\ &\quad (-6), 1)) \\ &\quad \quad \quad 4.519532140 \end{aligned} \quad (45)$$

```
> evalf(C3(1.042877508, 1.259860485, 0.01737451737,
1))
4.212006976 (46)
```

```
> evalf(C3(1.079779637, 1.410370323,
0.03441682600,1))
4.081481985 (47)
```

```
> evalf(C3(1.114294066, 1.538391756,
0.05247813411,1))
4.009354810 (48)
```

```
> evalf(C3(1.145720440, 1.645584376,
0.07107039918,1))
3.968512030 (49)
```

```
>
> evalf(C3(1.000011314, 1.064340602, 4.2826451*10^
(-6),10))
3.306673131 (50)
```

```
> evalf(C3(1.042877508, 1.259860485, 0.01737451737,
10))
3.123610966 (51)
```

```
> evalf(C3(1.079779637, 1.410370323,
0.03441682600,10))
3.050736784 (52)
```

```
> evalf(C3(1.114294066, 1.538391756,
0.05247813411,10))
3.011237510 (53)
```

```
> evalf(C3(1.145720440, 1.645584376,
0.07107039918,10))
2.989029167 (54)
```

```
> evalf(0.00001*ln(3/(2*Pi)))
-7.392647779 10-6 (55)
```

```
> Check := proc(c, r, eta)
    if       $-\frac{1}{2} < c - r$ 
        and  $c - r < 1 - c$ 
        and  $1 - c < -\text{eta}$ 
```



**and**  $-\eta < 0$

**and**  $0 < \frac{1}{4}$

**and**  $\frac{1}{4} \leq 2 \cdot c - c - \frac{\left(c - \frac{1}{2}\right)^2}{r} - \frac{1}{2}$

**and**  $2 \cdot c - c - \frac{\left(c - \frac{1}{2}\right)^2}{r} - \frac{1}{2} < \frac{1}{2}$

**and**  $\frac{1}{2} < 1$

**and**  $1 < 1 + \eta$

**and**  $1 + \eta < c$

**and**  $c < c + \frac{\left(c - \frac{1}{2}\right)^2}{r}$

**and**  $c + \frac{\left(c - \frac{1}{2}\right)^2}{r} < c + r$

**and**  $\text{theta}(c, r, 1 + \eta) < 2.1$

**then return** *true*;

**else return** *false*;

**end if**;

**end proc**;

*Check* := **proc**( $c, r, \eta$ )

**if**  $-1/2 < c - r$  **and**  $c - r < 1 - c$  **and**  $1 - c < -\eta$  **and**  $-\eta < 0$  **and**  $0 < 1/4$

(56)

```

and  $0 \leq c - (c - 1/2)^{2/r} - 3/4$  and  $c - (c - 1/2)^{2/r} < 1$  and  $1/2 < 1$  and  $0$ 
 $< \eta$  and  $\eta + 1 < c$  and  $c < c + (c - 1/2)^{2/r}$  and  $c + (c - 1/2)^{2/r} < c + r$  and
 $\theta(c, r, \eta + 1) < 2.1$  then

```

```

    return true

```

```

else

```

```

    return false

```

```

end if

```

```

end proc

```

```

> Check(1.000011314, 1.064340602, 4.2826451 * 10−6)

```

```

    true

```

(57)

```

> Check(1.042877508, 1.259860485, 0.01737451737)

```

```

    true

```

(58)

```

> Check(1.079779637, 1.410370323, 0.03441682600)

```

```

    true

```

(59)

```

> Check(1.114294066, 1.538391756, 0.05247813411)

```

```

    true

```

(60)

```

> Check(1.145720440, 1.645584376, 0.07107039918)

```

```

    true

```

(61)

```

>

```

```

>

```
